# Supplementary material for: Providing Access to Confidential Research Data Through Synthesis and Verification: An Application to Data on Employees of the U.S. Federal Government
Source: arXiv:1705.07872 ancillary file (2018-06-16)
Supplement: Supplementary file 1 [file SupplementA.pdf]

# Supplement A to "Providing Access to Confidential Research Data Trough Synthesis and Verification: An Application to Data on Employees of the U.S. Federal Government"

Andrés F. Barrientos, Alexander Bolton, Tom Balmat, Jerome P. Reiter, John M. de Figueiredo
Ashwin Machanavajjhala, Yan Chen, Charley Kneifel, Mark DeLong*

This document includes online supplementary material for the main text. In Section 1, we provide a formal description of the three sub-models used to model the employee's career. In Section 2, we discuss the modeling strategies used to synthesize several variables and to deal with some of the modeling challenges in the SF data. In Section 3, we provide the full list of the synthesized variables along with a brief description of each of them. In Section 4, we present the analyses of wage gaps conditional on six broad categories of occupation rather than the 803 used in the main text. In Section 5, we describe a method for empirical disclosure risk assessment for OPM synthetic data. In Section 6, we formally describe the verification measures for longitudinal trends in regression coefficients. In Section 7, we examine the performance of the $\epsilon$-differentially private described in Section 4.1 of the main text. In addition, we also present and examine the performance of a novel verification measure that is suitable for analyses where some regression coefficients are nonestimable

## 1 Model for Employees' Careers

We define an employee's career as the sequence of agencies where the employee has worked throughout the 24 years. Since most employees have not worked during all 24 years, these

*Andrés F. Barrientos is Postdoctoral Associate, Department of Statistical Science, Duke University, Durham, NC 27708 (email: afb26@stat.duke.edu); Alexander Bolton is Assistant Professor, Department of Political Science, Emory University, Atlanta, GA 30322 (abolton@emory.edu); Tom Balmat is Statistician, Social Science Research Institute, Duke University, Durham, NC 27708 (thomas.balmat@duke.edu); Jerome Reiter is Professor, Department of Statistical Science, Duke University, Durham, NC 27708 (jerry@stat.duke.edu); John de Figueiredo is Russell M. Robinson II Professor, Law School and Fuqua School of Business, Duke University, Durham NC 27708 (jdefig@duke.edu); Ashwin Machanavajjhala is Assistant Professor, Department of Computer Science, Duke University, Durham, NC 27708 (ashwin@cs.duke.edu); Yan Chen is Graduate Student, Department of Computer Science, Duke University, Durham, NC 27708 (yanchen@cs.duke.edu); Charley Kneifel is Senior Technical Director, Office of Information Technology, Duke University, Durham, NC 27701 (charley.kneifel@duke.edu); and, Mark DeLong is Director of Research Computing, Office of Information Technology, Duke University, Durham, NC 27701 (mark.delong@duke.edu). This research was supported by NSF grants ACI-14-43014 and SES-11-31897, as well as the Alfred P. Sloan Foundation grant G-2-15-20166003.

sequences do not always have the same length. This poses an additional challenge to be addressed when modeling this variable. To avoid this issue, we create an additional level for this variable. This level corresponds to the status not working. With this additional level, we only have to work with sequences of length equal to 24. Thus, the career of the $i$th employee is represented by

$$\mathbf{V}_1^i = (V_{1,1}^i, \ldots, V_{1,24}^i)$$

where $V_{1,t}^i$ denotes the agency where the $i$th employee worked in year $t$. To model these sequences, we create three additional variables: $G^i$, $\mathbf{Z}^i$, and $\mathbf{W}^i$, where

- $G^i$ is the number of agencies where the $i$th employee worked during the 24 years,
- $\mathbf{Z}^i = (Z_1^i, \ldots, Z_{G^i-1}^i)$ represents the list of years (minus one) when the $i$th employee moved to a new agency, and
- $\mathbf{W}^i = (W_1^i, \ldots, W_{G^i}^i)$ is the ordered sequence of agencies where the $i$th employee has worked.

Since that $(G^i, \mathbf{Z}^i, \mathbf{W}^i) \mapsto \mathbf{V}_1^i$ is a one-to-one mapping, we can equivalently define a model for either $(G^i, \mathbf{Z}^i, \mathbf{W}^i)$ or $\mathbf{V}_1^i$. Thus, we define a model for $\mathbf{V}_1^i$ by using $(G^i, \mathbf{Z}^i, \mathbf{W}^i)$ and an appropriate conditional representation. That is,

$$\begin{aligned}
\mathbb{P}\left[\mathbf{V}_1^i = \mathbf{v}\right] &= \mathbb{P}\left[(G^i, \mathbf{Z}^i, \mathbf{W}^i) = (g, \mathbf{z}, \mathbf{w})\right] \\
&= \mathbb{P}\left[\mathbf{W}^i = \mathbf{w} | (G^i, \mathbf{Z}^i) = (g, \mathbf{z})\right] \mathbb{P}\left[\mathbf{Z}^i = \mathbf{z} | G^i = g\right] \mathbb{P}\left[G^i = g\right],
\end{aligned}$$

with the following particular case,

$$\begin{aligned}
\mathbb{P}\left[\mathbf{V}_1^i = (v, v, \ldots, v)\right] &= \mathbb{P}\left[(G^i, \mathbf{W}^i) = (1, v)\right] \\
&= \mathbb{P}\left[\mathbf{W}^i = v | G^i = 1\right] \mathbb{P}\left[G^i = 1\right].
\end{aligned}$$

We propose to estimate $\mathbb{P}\left[G^i = g\right]$ and $\mathbb{P}\left[\mathbf{V}_1^i = (v, v, \ldots, v)\right]$ by using the corresponding observed frequencies. The estimators for the conditional models of $\mathbf{Z}^i$ and $\mathbf{W}^i$ are explained below.

## Model for $\mathbb{P}\left[\mathbf{Z}^i = \mathbf{z} | G^i = g\right]$

Henceforth we suppress the superscript $i$ for ease of notation. For sake of generality, we denote by $T$ the length of the employees' career. Conditional on $G$, we define the range of $Z$ as

$$\mathcal{P}_T^G := \left\{(a_1, \ldots, a_G) : a_1 < \ldots < a_G,\ (a_1, \ldots, a_G) \in \{1, \ldots, T-1\}^G\right\}.$$

For instance, if $T = 4$ and $G = 2$, then the range of $\mathbf{Z}$ corresponds to the set

$$\mathcal{P} = \{(1,2),(1,3),(1,4),(2,3),(2,4),(3,4)\}. \tag{1}$$

Notice that we can identify the space $\mathcal{P}_T^G$ with elements in the simplex space by considering the mapping,

$$\mathcal{P}_T^G \ni \mathbf{Z} = (Z_1, Z_2, \ldots, Z_G) \mapsto \mathbf{S} := \left(\frac{Z_1 - 1}{T-1}, \frac{Z_2 - Z_1 - 1}{T-1}, \ldots, \frac{Z_G - Z_{G-1} - 1}{T-1}\right) \in \Delta_G,$$

where $\Delta_G$ is the $G$-dimensional simplex space; that is,

$$\Delta_G = \left\{(a_1, \ldots, a_G) \in [0,1]^G : \sum_{j=1}^{G} a_j \leq 1\right\}.$$

In the example above, under this mapping, the set given in (1) is identified with the following set

$$\Delta = \left\{(0,0), \left(0, \frac{1}{3}\right), \left(0, \frac{2}{3}\right), \left(\frac{1}{3}, 0\right), \left(\frac{1}{3}, \frac{1}{3}\right), \left(\frac{2}{3}, 0\right)\right\}.$$

Let $\tilde{\mathbf{S}} = (\tilde{S}_1, \ldots, \tilde{S}_G)$ be a continuous latent random vector such that, conditioned on $G$, is $\Delta_G$-valued and

$$\mathbf{S} = \left(\frac{\lfloor (T-1)\tilde{S}_1 \rfloor}{T-1}, \ldots, \frac{\lfloor (T-1)\tilde{S}_G \rfloor}{T-1}\right).$$

Thus, we define a probability model for $\mathbf{Z}$, conditional on $G$, of the form

$$\begin{aligned}
&\mathbb{P}\left[\mathbf{Z} = \mathbf{z} \middle| G = g\right] \\
&= \mathbb{P}\left[\mathbf{S} = \left(\frac{z_1 - 1}{T-1}, \frac{z_2 - z_1 - 1}{T-1}, \ldots, \frac{z_g - z_{g-1} - 1}{T-1}\right) \middle| G = g\right], \\
&= \mathbb{P}\left[\tilde{\mathbf{S}} \in \left(\frac{z_1 - 1}{T-1}, \frac{z_1}{T-1}\right] \times \left(\frac{z_2 - z_1 - 1}{T-1}, \frac{z_2 - z_1}{T-1}\right] \times \ldots \times \right. \\
&\qquad \left. \left(\frac{z_g - z_{g-1} - 1}{T-1}, \frac{z_g - z_{g-1}}{T-1}\right] \middle| G = g\right].
\end{aligned}$$

Since $\tilde{\mathbf{S}}$ is a continuous random vector on the simplex, we assume that its corresponding probability measure is absolutely continuous with respect to the Lebesgue measure with density $f_{\tilde{\mathbf{S}}}$. This probability density function is assumed to be a mixture of Dirichlet densities of the form,

$$f_{\tilde{\mathbf{S}}}(\tilde{\mathbf{s}} | G = g, \boldsymbol{\pi}, \boldsymbol{\alpha}) = \sum_{\mathbf{j} \in \mathcal{P}_T^g} \mathbf{p_j} \mathrm{dir}_g\left(\tilde{\mathbf{s}} \,|\mathbf{a_j}\right)$$

where $\boldsymbol{\pi} = (\mathbf{p_j})_{\mathbf{j} \in \mathcal{P}_T^g}$ denotes the weights, $\mathrm{dir}_g(\cdot|\mathbf{a})$ stands for a $g$-dimensional Dirichlet density with parameters $\mathbf{a}$, and $\boldsymbol{\alpha} = (\mathbf{a_j})_{\mathbf{j} \in \mathcal{P}_T^g}$. The number of components of this mixture is equal to

the cardinality of $\mathcal{P}_T^g$, i.e., equal to the number of elements in the range of $\mathbf{Z}$.

Models designed to generate synthetic datasets should have parameters that allow users to control the trade-off between privacy and statistical usefulness. For this reason, we propose to estimate the parameter $\boldsymbol{\pi}$ and use a deterministic definition for $\boldsymbol{\alpha}$. Specifically, we propose to estimate $\boldsymbol{\pi}$ using the empirical frequencies, i.e.,

$$\hat{\mathbf{p}}_{\mathbf{j}} = \hat{\mathbf{p}}_{\{j_1, j_2, \ldots, j_g\}} \propto \sum_{i \in \{l : G_i = g\}} \mathbb{I}_{\{Z_1^i = j_1, \ldots, Z_g^i = j_g\}}.$$

Instead of using frequentist estimation of $\boldsymbol{\pi}$, we could also place a prior distribution on $\boldsymbol{\pi}$ and provide an estimation through the posterior distribution. Regarding the parameter $\boldsymbol{\alpha}$, we propose the following definition.,

$$\mathbf{a}_{\mathbf{j}} = \theta \left(2j_1 - 1, 2(j_2 - j_1) - 1, \ldots, 2(j_{g-1} - j_g) - 1, 2(T-1) - 2j_g + g\right),$$

where $\theta$ is a positive constant. If the parameters $\boldsymbol{\pi}$ and $\boldsymbol{\alpha}$ are defined as before, then the overfitting and underfitting of the model can be controlled by $\theta$. Notice that if a model overfits the confidential dataset, then the synthetic dataset obtained from that model should be very similar to the confidential dataset. Hence, overfitting implies high statistical usefulness but low privacy level. Under a analogous reasoning, we can associate the underfitting with low statistical usefulness but high privacy level. Thus, under this parametrization, the mean and the variance of a Dirichlet distribution with parameter $\mathbf{a}_{\mathbf{j}}$ are equal to

$$\left(\frac{2j_1 - 1}{2(T-1)}, \frac{2(j_2 - j_1) - 1}{2(T-1)}, \ldots, \frac{2(j_g - j_{g-1}) - 1}{2(T-1)}\right),$$

and

$$\left(\frac{2(j_l - j_{l-1})\theta[2(T-1)\theta - g - 2(j_l - j_{l-1})\theta]}{[2(T-1)\theta - g]^2[2(T-1)\theta - g + 1]}\right)_{l=1}^{g},$$

respectively. Notice that this mean always belongs to the inner of the hypercube defined by

$$\mathcal{I}_{\mathbf{j}} := \left(\frac{j_1 - 1}{T-1}, \frac{j_1}{T-1}\right] \times \left(\frac{j_2 - j_1 - 1}{T-1}, \frac{j_2 - j_1}{T-1}\right] \times \ldots \times \left(\frac{j_g - j_{g-1} - 1}{T-1}, \frac{j_g - j_{g-1}}{T-1}\right],$$

and notice too that the variance goes to 0 when $\theta \to \infty$. The above statements imply that

$$\mathbb{P}\left[Z = z \,|\, G = g, \theta, \text{Data}\right] = \sum_{\mathbf{j} \in \mathcal{P}_T^g} \hat{\mathbf{p}}_{\mathbf{j}} \int_{\mathcal{I}_{\mathbf{z}}} \text{dir}_g\left(\tilde{\mathbf{s}} \,|\mathbf{a}_{\mathbf{j}}\right) d\tilde{\mathbf{s}} \underset{\theta \to \infty}{\longrightarrow} \hat{\mathbf{p}}_{\mathbf{z}},$$

meaning that if $\theta$ increases, the latent model assigns probability equal to $\hat{p}_{\mathbf{j}}$ to the hypercube $\mathcal{I}_{\mathbf{j}}$ (i.e., overfitting). On the other hand, when $\theta$ decreases, the model borrows information across all the hypercubes $\{\mathcal{I}_{\mathbf{j}}\}_{\mathbf{j} \in \mathcal{P}_T^g}$ (i.e., underfitting). The information related to an specific hypercube $\mathcal{I}_{\mathbf{j}}$

is borrowed across the other hypercubes. The amount of borrowed information depends on the distance between $\mathcal{I}_{\mathbf{j}}$ and the other hypercubes. The smaller the distance, the larger the amount of borrowed information. In particular, if $\theta$ is small enough, most of the information will be transferred to the other hypercubes. This increases the probability of generating new careers for the synthetic employees that do not match with the careers of the confidential employees. In other words, if $\theta$ is small, it can lead to a degradation of the statistical information contained in a synthetic data, but also an improvement in terms of privacy. Under this model, $\theta$ is the parameter controlling the trade-off between statistical usefulness and privacy level.

### Model for $\mathbb{P}[\mathbf{W} = \mathbf{w} | (G, \mathbf{Z}) = (g, \mathbf{z})]$

Under some assumptions of independence, we simplify the definition of this model. Specifically, we assume that

$$\begin{aligned}
\mathbb{P}[\mathbf{W} = \mathbf{w} | (G, \mathbf{Z}) = (g, \mathbf{z})] \quad \propto \quad & \mathbb{P}[\mathbf{W} = \mathbf{w}, G = g, \mathbf{Z} = \mathbf{z}] \\
:= \quad & \mathbb{P}[W_1 = w_1 | G = g, Z_1 = z_1] \\
& \times \mathbb{P}[W_2 = w_2 | W_1 = w_1, G = g, Z_1 = z_1, Z_2 = z_2] \\
& \times \prod_{j=3}^{g} \mathbb{P}[W_j = w_j | W_{j-1} = w_{j-1}, G = g, Z_j = z_j, Z_{j-1} = z_{j-1}, Z_{j-2} = z_{j-2}] \\
& \times \mathbb{P}\left[W_{g+1} = w_{g+1} | W_g^i = w_g, G = g, Z_g = z_g, Z_{g-1} = z_{g-1}\right], \\
= \quad & \mathbb{P}[W_1 = w_1 | G = g, Z_1 = z_1] \\
& \times \prod_{j=2}^{g+1} \mathbb{P}[W_j = w_j | W_{j-1} = w_{j-1}, G = g, Y_j = y_j]
\end{aligned} \tag{2}$$

where $\mathbf{Z} \mapsto (\mathbf{Y}_2, \ldots, \mathbf{Y}_{g+1})$ is a one-to-one transformation and

$$\mathbf{Y}_j = (Y_{j,1}, Y_{j,2}, Y_{j,3}) = \begin{cases} (0, Z_1 - 1, Z_2 - Z_1 - 1) & \text{if } j = 2, \\ (Z_{j-2} - 1, Z_{j-1} - Z_{j-2} - 1, Z_j - Z_{j-1} - 1) & \text{if } j = 3, \ldots, g, \\ (Z_{g-1} - 1, Z_g - Z_{g-1} - 1, T - Z_g) & \text{if } j = g + 1. \end{cases}$$

Notice that $Y_j$ is related to the moments where the transition $w_{j-1} \to w_j$ is made. The first component of this random vector represents the year (minus one) when the employee started to work for agency $w_{j-1}$. The second and third components indicate for how many years (minus one) the employee worked for agency $w_{j-1}$ and $w_j$, respectively. Since the terms in (2) can be

re-written of the form,

$$\begin{aligned}
&\mathbb{P}\left[W_1 = w_1 | G = g, Z_1 = z_1\right] \;\propto\; \mathbb{P}\left[W_1 = w_1, G = g, Z_1 = z_1\right], \\
&= \sum_{z_2=z_1+1}^{23-g-2} \sum_{w_2 \in \mathcal{A}_{z_2+1}} \mathbb{P}\left[Z_1 = z_1, Z_2 = z_2 | W_2 = w_2, W_1 = w_1, G = g\right] \mathbb{P}\left[W_2 = w_2, W_1 = w_1, G = g\right], \\
&= \sum_{z_2=z_1+1}^{23-g-2} \sum_{w_2 \in \mathcal{A}_{z_2+1}} \mathbb{P}\left[\mathbf{Y}_2 = (0, z_1 - 1, z_2 - 1) | W_2 = w_2, W_1 = w_1, G = g\right] \times \\
&\qquad\qquad\qquad\qquad\qquad\qquad\qquad\qquad \mathbb{P}\left[W_2 = w_2, W_1 = w_1, G = g\right],
\end{aligned}$$

and

$$\begin{aligned}
\mathbb{P}\left[W_j = w_j | W_{j-1} = w_{j-1}, G = g, \mathbf{Y}_j = \mathbf{y}_j\right] &\propto \mathbb{P}\left[W_j = w_j, W_{j-1} = w_{j-1}, G = g\right] \\
&\times \mathbb{P}\left[\mathbf{Y}_j = \mathbf{y}_j | W_j = w_j, W_{j-1} = w_{j-1}, G = g\right],
\end{aligned}$$

we propose to estimate the terms $\mathbb{P}\left[W_j = w_j, W_{j-1} = w_{j-1}, G = g\right]$ using the observed frequencies. We denoted by $\mathcal{A}_t$ as the set of all existing agencies at year $t$. We could also estimate these probabilities through a multinomial-Dirichlet Bayesian model. For the term $\mathbb{P}\left[\mathbf{Y}_j = \mathbf{y}_j | W_j = w_j, W_{j-1} = w_{j-1}, G = g\right]$, we use the same latent model defined described in the previous subsection. This is possible because $\mathbf{Y}_j/(T-G) = (Y_{1,j}, Y_{2,j}, Y_{3,j})/(T-G)$ lies in the three-dimensional simplex space. Thus, let $\tilde{\mathbf{Y}}_j = (\tilde{Y}_{1,j}, \tilde{Y}_{2,j}, \tilde{Y}_{3,j})$ be a $\Delta_3$-valued continuous latent random vector such that, conditional on $G$,

$$\mathbf{Y}_j = \left(\lfloor (T-M)\tilde{Y}_{1,j} \rfloor, \lfloor (T-M)\tilde{Y}_{2,j} \rfloor, \lfloor (T-M)\tilde{Y}_{3,j} \rfloor\right).$$

We define a probability model for $\mathbf{Y}_j$, conditional on $W_j$, $W_{j-1}$, and $G$, of the form

$$\begin{aligned}
&\mathbb{P}\left[\mathbf{Y}_j = (y_{1,j}, y_{2,j}, y_{3,j}) \middle| W_j = w_j, W_{j-1} = w_{j-1}, G = g\right] \\
&= \mathbb{P}\left[\tilde{\mathbf{Y}}_j \in \left(\frac{y_{1,j}}{T-1}, \frac{y_{1,j}+1}{T-1}\right] \times \left(\frac{y_{2,j}}{T-1}, \frac{y_{2,j}+1}{T-1}\right] \times \right. \\
&\qquad\qquad\qquad\qquad \left. \left(\frac{y_{3,j}}{T-1}, \frac{y_{3,j}+1}{T-1}\right] \middle| W_j = w_j, W_{j-1} = w_{j-1}, G = g\right].
\end{aligned}$$

We also assume that the law of $\tilde{\mathbf{Y}}_i$ has a probability density function and is defined as a mixture of Dirichlet densities of the form,

$$f_{\tilde{Y}_j}(\tilde{y} | W_j = w_j, W_{j-1} = w_{j-1}, G = g, \boldsymbol{\pi}', \boldsymbol{\alpha}') := \sum_{\mathbf{j} \in \mathcal{P}^3_{T-g}} \mathbf{p}'_{\mathbf{j}} \mathrm{dir}_3\left(\tilde{\mathbf{y}} \left| \mathbf{a}'_{\mathbf{j}}\right.\right)$$

where $\boldsymbol{\pi}' = (\mathbf{p}'_{\mathbf{j}})_{\mathbf{j} \in \mathcal{P}^3_{T-g}}$ and $\boldsymbol{\alpha}' = (\mathbf{a}'_{\mathbf{j}})_{\mathbf{j} \in \mathcal{P}^3_{T-g}}$. Since our goal is still the same, i.e., to propose models that provide control over the trade-off between privacy and statistical usefulness, the parameters $\boldsymbol{\pi}'$ and $\boldsymbol{\alpha}'$ are estimated and defined in a similar manner to the one proposed in the

previous subsection. Specifically,

$$\hat{\mathbf{p}}'_{\{j_1,j_2,j_3\}} \propto \sum_{\substack{j=2,\ldots,g+1 \\ i \in \{l : G^i_l = g, W^i_j = w_j, W^i_{j-1} = w_{j-1}\}}} \mathbb{I}_{\left\{Y^i_{1,j}=j_1-1, Y^i_{2,j}=j_2-j_1-1, Y^i_{3,j}=j_3-j_2-1\right\}}.$$

and

$$\mathbf{a}'_{\mathbf{j}} = \theta\left(2j_1 - 1, 2(j_2 - j_1) - 1, 2(j_3 - j_2) - 1, 2(T - g) - 2j_3 + 3\right).$$

Here, the implications of increasing or decreasing the value of $\theta$ remain the same as in the previous subsection.

# 2 General Strategies for Synthesizing the OPM Dataset

The modeling of the SF dataset requires us to deal with many non-trivial problems. For each of these problems, we design different strategies that take run time and computational resources into account. In this section, we provide a more detailed description of the most relevant strategies proposed during the modeling of the SF dataset.

## 2.1 Deriving predictors from employees' careers

After generating the synthetic careers, we create a set of variables that are functions of the employees' careers. These variables serve as predictors in the modeling of the remaining variables in the SF dataset. Specifically, we create the following variables.

- *Initial year*: year when the employee was included in the dataset.
- *Last year*: year in which the employee stopped working in the last agency.
- *Total years*: number of years that the employee worked.
- *Initial agency*: agency in which the employee started working.
- *Number of moves*: number of times that the employee changed agency during her/his career.
- *Number of gaps*: number of times that the employee stopped working for at least one year and then started working again.

## 2.2 General strategy for static variables

Static variables are those variables whose values remain the same across time. We model these variables using classification and regression trees (CART), as described in Reiter (2005). For

each static variable, we use as predictors the variables derived from the employees' careers along with all the original values of the variables previously synthesized. The sex and a binary variable associated with months of military service are classified in this category.

### 2.3 General strategy for longitudinal variables

Longitudinal variables are those variables that do not change deterministically across time. Let $t_1^i < \ldots < t_{n_i}^i$ be the years when $i$th employee is observed and $\mathbf{V}_j^i := (V_{j,t_1^i}^i, \ldots, V_{j,t_{n_i}^i}^i)$. If $\mathbf{V}_j^i$ is a longitudinal variable, $j > 1$, then we consider the following conditional representation of $p_j$,

$$p_j\left(\mathbf{V}_j^i \left|\mathbf{V}_1^i, \ldots, \mathbf{V}_{j-1}^i\right.\right) := \prod_{l=1}^{n_i} p_{j,t_l^i}\left(\mathbf{V}_{j,t_l^i}^i \middle| \mathbf{V}_1^i, \ldots, \mathbf{V}_{j-1}^i, V_{j,t_1^i}^i, \ldots, V_{j,t_{l-1}^i}^i\right) \tag{3}$$

where $p_{j,t_l^i}$ denotes the distribution $V_{j,t_l}^i$ which is conditioned on the values of the previous variables and the past values of $\mathbf{V}_j^i$, i.e., $V_{j,t_1^i}^i, \ldots, V_{j,t_{l-1}^i}^i$. In order to simply the modeling of $p_{j,t_l^i}$, we assume that

$$p_{j,t_l^i}\left(V_{j,t_l^i}^i \middle| \mathbf{V}_1^i, \ldots, \mathbf{V}_{j-1}^i, V_{j,t_1^i}^i, \ldots, V_{j,t_{l-1}^i}^i\right) = p_{j,t_l^i}\left(V_{j,t_l^i}^i \middle| V_{1,t_l^i}^i, \ldots, V_{j-1,t_l^i}^i, V_{j,t_{l-1}^i}^i\right), \tag{4}$$

This assumption implies that the conditional distribution of $V_{j,t_l^i}^i$ only dependents of current values of $\mathbf{V}_l^i$, $1 < l < j$, and the nearest past value of $\mathbf{V}_j^i$. We estimate these conditional probabilities using CART models.

### 2.4 General strategy for variables with a high proportion of constant sequences

There are variables whose values do not change across time for most employees. Specifically, race and educational level show this pattern. For this reason, we create an auxiliary binary variable that indicates whether the values of the variable remain the same across time or not. After imputing this binary variable to the synthetic employees using CARTs, we divide the dataset into two groups. The first group represents those employees whose values remain the same across time. This group is modeled using the general strategy for static variables. The second group represents those employees whose values change across time. We model this group using the general strategy for longitudinal variables.

### 2.5 General strategy for oddities

Some observations have values that are theoretically impossible. For example, for any given employee, we expect the values associated with educational level are not decreasing. However, we observe that there are some employees whose educational level drops at some point. We

assume that a drop in the educational level should be considered as an oddity. The SF synthetic dataset represents a methodological tool for those researches that will only have access to the original dataset for a limited period of time. For those researchers, the synthetic dataset can be used to define which models they plan to run when they have access to the original dataset. Hence, fitting a model to the synthetic data should lead to similar challenges to the ones the researches will face when they access the original dataset. For this reason, we define a model able to generate those oddities. To do so, we create a binary variable that indicates whether the employee contains an oddity or not. Thus, we use this binary variable to fit a CART model that allows us to classify the synthetic employees in two groups. The first is the group that is synthesized with a model that does not generate oddities, i.e., a model that only generates non-decreasing sequences. The second is a group that is synthesize with a model that generates oddities with positive probability.

## 2.6 General strategy for bucketed continuous variables

Age and yrsdegrng—years since the employee earned the degree mentioned in educational level—are classified in this category. The levels of these variables are reported in 5-year buckets. For this reason, we model age and yrsdegrng as categorical variables using the first reported bucket as a response variable. Thus, we synthesize these variables using the general strategy for static variables. Once we impute the first age and yrsdegrng to the synthetic employee, we deterministically impute the values of the next years using the middle of the range of the buckets. For example, we impute $a_t$—age in year $t$—by adding one to the mid-range value in the previous year $a_{t-1}$; that is, $a_t = a_{t-1} + 1$. Finally, we bucket the imputed values back into 5-year buckets.

## 2.7 General strategy for variables with a large number of levels

Fitting a CART using a response variable with a large number of levels requires a high computational cost. In fact, the R function tree only allows a response variable with at most 32 levels. To wave this issue, we create an auxiliary variable that is a copy of the original variable with only 32 levels, where the first 31 levels correspond to those levels with the highest observed frequencies and the last level groups the remaining levels. Then we fit a CART model to this auxiliary variable and predict the values for the synthetic employees. Thus, there are some synthetic employees having the value associated with the last level of the auxiliary variable. For those employees, we re-impute their values using a CART fitted to a new auxiliary variable. This CART is fitted to a subset of the original dataset that does not contain those employees whose values correspond to one of the 31 levels with most data points. This new auxiliary variable also has 32 levels. The first 31 levels correspond to those levels with most data points in such subset and the last level grouped the rest of the levels. We repeat this process until we reach

those levels with the smallest observed frequencies.

## 2.8 General strategy for variables with low observed frequency levels

This strategy is used for occupation. This variable has over eight hundred levels each year. Some of these occupations have a very low observed frequency. Therefore, the probability that we impute one of these occupations to a synthetic employee is also small. In fact, we observe that, after having used the general strategy for variables with a large number of levels, there are some occupations in the synthetic data with an observed frequency equal to zero. The absence of these occupations is problematic for those researchers interested in occupations with small frequency. In other words, it would be useless for them to have a synthetic dataset where some of these occupations do not appear. To deal with this issue, we start modeling this variable by using the general strategy for variables with a large number of levels. Thus, we guarantee that those occupations with a large number of data points are reasonably represented in the synthetic dataset. For those occupations with a small number of observations, we use propensity score matching. Specifically, we combine the synthetic and original datasets into one dataset. Then, we fit a logistic regression model using whether the employee is a synthetic one or not as a response variable. We use the predicted probabilities to match synthetic employees with authentic employees having an occupation that has a small observed frequency. Thus, the synthetic employee is assigned to the same occupation of the corresponding matched authentic employee.

## 2.9 General strategy for structural zeros

We define a structural zero as an impossible combination of levels of different variables. For example, if we have age and educational level, the combination one-year-old and college degree should occur with a probability equal to zero. Defining models for a categorical response that deal with structural zeros is a difficult task. This task can be even more difficult if there is no exhaustive list of these impossible combinations. Structural zeros can occur if we do not carefully model some of the variables in the SF dataset. For example, there are occupations absent in certain agencies or some grades that only make sense within a particular pay plan. The strategy we use here is to split the dataset into subsets such that if we fit a CART model to that subset, the CART model will not impute values that produce structural zeros. Specifically, we always split the data at least into agency. However, for some variables, we require dividing the dataset considering other variables. For example, we know that the levels that grade can take are restricted by the pay plan. In this case, we have to divide the dataset not only by agency but also by pay plan.

### 2.10 General strategy for missing values

Almost all variables of the SF dataset have missing values. To deal with this aspect, we assume that the missing status is an additional level that each variable can take. Hence, under this strategy, models fitted to the confidential dataset are able to generate synthetic employees with missing values. This leads to synthetic datasets more similar to the confidential one regarding the presence of missing values. Thus, users can design modeling strategies that account for missing data using the synthetic dataset. These strategies could potentially be implemented in the confidential dataset if the user plans to access it in the future.

Another strategy to deal with missing data is imputation. In this work, we impute a missing value if a deterministic rule can provide a reasonable approximation of the unobserved value. We can think of this strategy more as a cleaning step than as a formal statistical procedure to deal with missing values. This strategy is used in only one variable, educational level. The rules that we consider for this specific variable are:

- If the initial educational levels are missing, we impute those with the first reported educational level.
- If the last educational levels are missing, we impute those with the last reported educational level.
- If the educational level is reported at year $t_1$ and $t_2$, with $t_1 < t_2$, and the values of this variable are missing for every year $t \in \{t_1 + 1, \dots, t_2 - 1\}$, then we impute those missing values with the educational level reported at year $t_1$.

Notice that, under these rules, some employees can still have missing values in this variable. Specifically, those employees for whom all the educational level values are missing will not be assigned any values for educational level after the imputation. To deal with this issue, as before, we model this variable assuming that the missing status corresponds to an additional educational level.

### 2.11 General strategy for allowances

For each year, we create a binary variable to predict whether or not the synthetic employee receives an allowance. We model these binary sequences using the general strategy for longitudinal variables. Then, for each year and using those authentic employees that have received an allowance, we compute how much this allowance is as a percentage of basic pay. This creates a population of percentages related to the allowances received by the employees each year. If a synthetic employee is classified as receiving an allowance, then we compute this allowance by multiplying her basic pay by a percentage randomly drawn from the percentage population of the corresponding year.

# 3 List of Synthesized Variables

In this section, we provide a full list of the synthesized variables. The variables in this list are ordered from the first to last to be synthesized.

1. **Agency**. Each entry of personnel data from the Central Personnel Data File (CPDF) is accompanied by a distinct agency identifier (e.g., AG13 or HUAA). These 4-digit codes are a combination of letters and numbers. The first two digits signify the overarching agency (e.g., AG=Department of Agriculture) and the last two digits signify a sub-element within the agency if there is one (e.g., Forest Service).

2. **Sex**. An employee's sex.

3. **Race**. Race or National Origin - An employee's race or national origin. Employees of mixed race or national origin should be identified with the race or national origin with which they most closely associate themselves. This data standard is only applicable to an employee whose accession occurs prior to July 1, 2006. See the ETHNICITY AND RACE IDENTIFICATION data standard for an employee whose accession occurs on or after January 1, 2006.[1]

4. **Eribridge**. The data standard is applicable to accessions occurring on or after January 1, 2006, and is required for accessions occurring on or after July 1, 2006. The data standard consists of one ethnicity category (Hispanic or Latino) and five race categories.

5. **Educ_lvl**. The extent of an employee's educational attainment from an accredited institution.[2]

6. **Agerange**. The age of the employee in the year observed within a particular range. The method to generate the variable is as follows: OPM took the real age, randomly added error, which is uniformly distributed around 0 and goes from -2 to +2. That generates a predicted age, which is then bucketed into 5-year buckets. The variable agerange is the predicted age in the 5-year bucket. This is generated year-by-year, not person-by-person.

7. **Yrsdegrng**. Years since the employee earned the degree mentioned in educ_lvl. OPM took the real year, randomly added error, which is uniformly distributed around 0 and goes from -2 to +2. That generates a predicted year, which is then bucketed into 5-year buckets. The variable yrsdegrng is the predicted number of years in the 5-year bucket. This is generated year-by-year, not person-by-person.

[1] The Guide to Data Standards, Update 16, November 15, 2014, A-420.
[2] The Guide to Data Standards, Update 16, November 15, 2014, A-130.

8. **Milmonths**. The months of military service that are creditable for annual leave accrual purposes. This variable was generated using the milserve (same as CREDIBLE MILITARY SERVICE) variable provided to us by OPM.[3]

9. **Occ**. Occupation - An employees occupational series. Occupational Series 0001 through 2299 represent white collar occupations and occupational series 2501 through 9999 represent blue collar occupations.[4]

10. **Instrctpgm**. Instructional Program - an employees field of study.[5]

11. **Occ_cat**. Occupational Category - The occupational category to which an occupational series belongs.[6]

12. **Funcclas**. Functional Class - An employee's primary work function as a scientist or engineer.

13. **Flsa**. The status of a Federal civilian employee under the authority of Section 13 of the Fair Labor Standards Act (29 U.S.C. 213), as amended.

14. **Appttype**. Type of Appointment  the type of appointment under which an employee is serving.[7]

15. **Polappttype**. Political Appointment Type. - Political appointee is a generic term that is not defined in OPM staffing policy. For purposes of our analyses a political appointee, non-career SES employee, or Schedule C employee who can be identified as such in OPMs Central Personnel Data File (CPDF) or Enterprise Human Resources Integration-Statistical Data Mart (EHRI-SDM).

16. **Position**. Position Occupied  an employee's position in the Competitive Service, Excepted Service, or the Senior Executive Service.[8]

17. **Tenure**. For purposes of reduction in force, the retention group in which an employee is placed based on the employee's type of appointment.[9]

18. **Svsrstat**. Supervisory status - The nature of managerial, supervisory, or non-supervisory responsibility assigned to an employee's position.[10]

[3]The Guide to Data Standards, Update 16, November 15, 2014, A-86.
[4]The Guide to Data Standards, Update 16, November 15, 2014, A-307.
[5]The Guide to Data Standards, Update 16, November 15, 2014, A-173-A-236.
[6]The Guide to Data Standards, Update 16, November 15, 2014, A-343.
[7]The Guide to Data Standards, Update 16, November 15, 2014, A-510.
[8]The Guide to Data Standards, Update 16, November 15, 2014, A-396.
[9]The Guide to Data Standards, Update 16, November 15, 2014, A-506  A-507.
[10]The Guide to Data Standards, Update 16, November 15, 2014, A-504  A-505.

19. **Bargunit**. An employee's bargaining unit. Bargaining unit names and codes can be found in the Office of Personnel Managements Federal Labor Management Information System (FLIS) website (https://apps.opm.gov/flis/start.aspx).[11]

20. **Pay_plan**. A particular table or array of pay rates prescribed by law or other authoritative source that establishes the basic pay rates for certain employees. In most cases, a pay plan (system) is a two dimensional matrix of pay rates: one dimension providing a series of different pay rates or ranges corresponding to differences in grade (or level, class, rank, or pay band of work) and the other dimension providing a series of pay rates or a range of rates within a grade. These rates may be a function of length of service in the grade or of performance ratings.[12]

21. **Grade**. An indicator of hierarchical relationships among positions covered by the same pay plan or system.[13]

22. **Steprate**. An indicator of a specific salary within a grade, level, class, rate, or pay band.

23. **Paybasis**. The principal condition in terms of time, production, or other criteria that, along with salary rate, determines the compensation paid to an employee.

24. **Workschd**. Work Schedule - The time basis on which an employee is scheduled to work.

25. **Payrated**. A designation of any special factors that help determine an employee's rate of basic pay or adjusted basic pay.[14]

26. **Localpay**. Locality Pay Area - the identification of an area for purposes of locality-based comparability payments.

27. **Paybasic**. The employees rate of basic pay. Exclude supplements, adjustments, allowances, differentials, incentives, or other similar additional payments.

28. **Retallow**. This variable comes from Nature of Action code 827, Retention Incentive.[15]

29. **Svsr_diff**. Supervisory Differential - The annual total dollar amount paid, over and above paybasic, to a General Schedule supervisor who otherwise would be paid less than one or more of the civilian employees supervised.[16]

[11] The Guide to Data Standards, Update 16, November 15, 2014, A-59.
[12] The Guide to Data Standards, Update 16, November 15, 2014, A-352 A-386.
[13] The Guide to Data Standards, Update 16, November 15, 2014, A-168 A-169.
[14] The Guide to Data Standards, Update 16, November 15, 2014, A-387 A-392.
[15] The Guide to Data Standards, Update 16, November 15, 2014, A-302.
[16] The Guide to Data Standards, Update 16, November 15, 2014, A-503.

| Variable | Males' Regression Synthetic | Males' Regression Confidential | Females' Regression Synthetic | Females' Regression Confidential |
|---|---|---|---|---|
| AI/AN | -.016 (9) | -.034 (17) | -.017 (11) | -.036 (21) |
| Asian | -.014 (11) | -.027 (20) | .004 (4) | .014 (12) |
| Black | -.058 (86) | -.083 (116) | -.009 (20) | -.011 (23) |
| Hispanic | -.016 (20) | -.033 (37) | -.014 (17) | -.018 (22) |
| | | | | |
| Employee-years | 13,008,298 | 12,720,500 | 12,263,514 | 11,874,048 |
| Employees | 1,446,499 | 1,430,238 | 1,390,611 | 1,348,381 |

Table 1: Coefficients from overall regression models. AI/AN stands for American Indian and Alaska Native, and Asian includes individuals that identify as Native Hawaiian or Pacific Islander. Absolute values of $t$-statistics are in parentheses. Disparities in sample sizes arise from deletions of cases with missing values in the confidential data analyses. These models include an indicator for an individual's occupational category code – professional, administrative (omitted category), technical, clerical, other white collar, or blue collar. Models also include controls for age, age squared, and educational attainment.

## 4 Results for Model With Broad Occupation Classification

Table 1 includes estimates of the racial wage gap over the 1988-2011 time period for men and women from the synthetic and authentic datasets. These estimates are from models similar to those reported in the main text of the paper. However, rather than including indicators for disaggregated occupational information, we use indicators for broad occupational indicators created by the Office of Personnel Management. There are six possible categories: administrative (omitted group), blue collar, clerical, other white collar, professional, and technical.

In general, administrative jobs require a college degree and are primarily white collar positions with management functions. This is the largest category of positions in the federal government. Professional positions tend to be complex and technical in function, requiring advanced degrees and training. Examples would include engineers and scientists. Clerical positions and technical positions tend to be supportive roles within agencies that do not require a bachelor's degree and/or individuals may be able to be trained on the job. These categories include positions like administrative assistants (clerical) and nursing assistants (technical). Blue collar positions have shrunk in number over time, but they include trades and craft workers in both supervisory and non-supervisory roles. Finally, other white collar positions include those that do not comfortably fall into any of the other white collar categories, such as student trainees for a variety of white collar positions or border patrol enforcement (Office of Personnel Management, 2014).

If individuals' races play an important role in the specific occupations that they work in, then conditioning on occupational information could induce post-treatment bias in our estimates of the racial wage gap. Race may play a role, for example, if there is significant racial discrimination

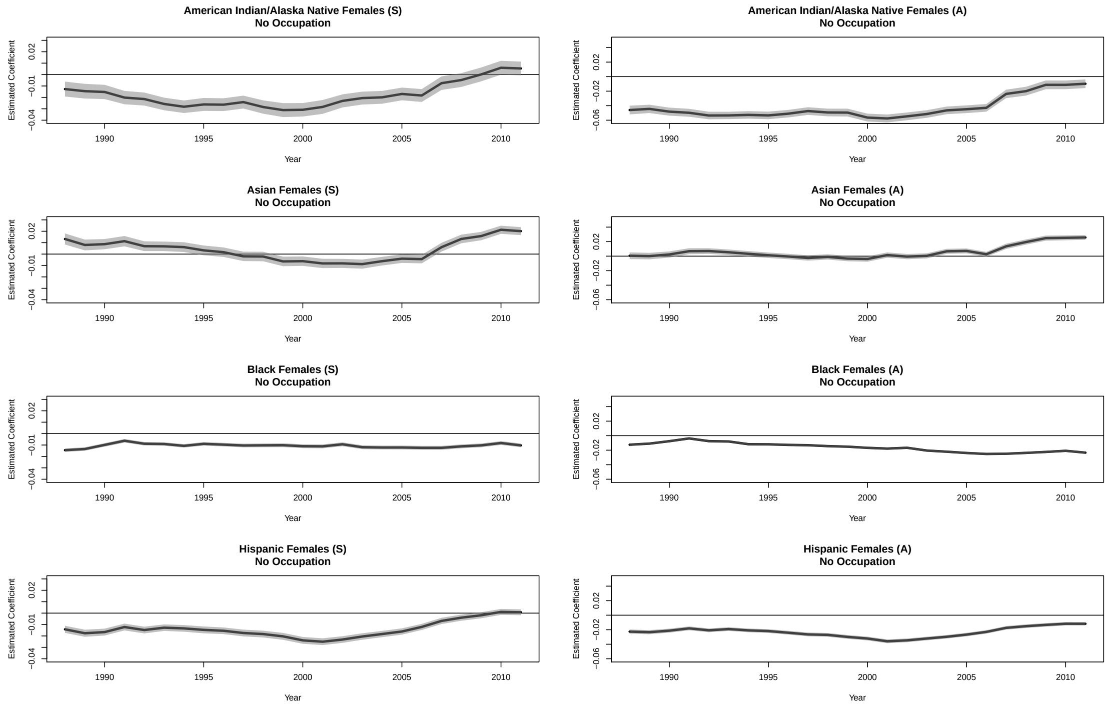


Figure 1: Estimated racial wage gaps (coefficients of race indicators) for yearly females' regressions in synthetic data (left) and confidential, authentic data (right). These models include an indicator for an individual's occupational category code – professional, administrative (omitted category), technical, clerical, other white collar, or blue collar.

or legacies of discrimination in particular occupations or classes of occupations. In that case, conditioning on occupation would not give a full picture of racial pay disparities. However, completely excluding occupational information may lead to incorrect inferences if occupational sorting rather than discrimination is at play. Here, we "split the difference," by including only broad occupational information. Results with no occupational indicators in models are available upon request.

As can be seen in Table 1, the estimated wage gaps are in general larger than those reported in the main text of the paper when including more aggregated occupational indicators. In all cases, except for Asian female employees, we see an estimated negative coefficient for each group, indicating that they are paid less than comparable white employees. These signed relationships are found in both the synthetic and the confidential datasets, although the coefficients estimated from the confidential dataset tend to be of larger magnitude.

Figure 1 displays the over-time trends in estimated racial pay gaps with 95% confidence intervals for female employees in the synthetic and confidential datasets, respectively. Both figures show similar trends both to one another, as well as to those reported in the main text of the paper. The key place in which the synthetic and confidential datasets depart in their results

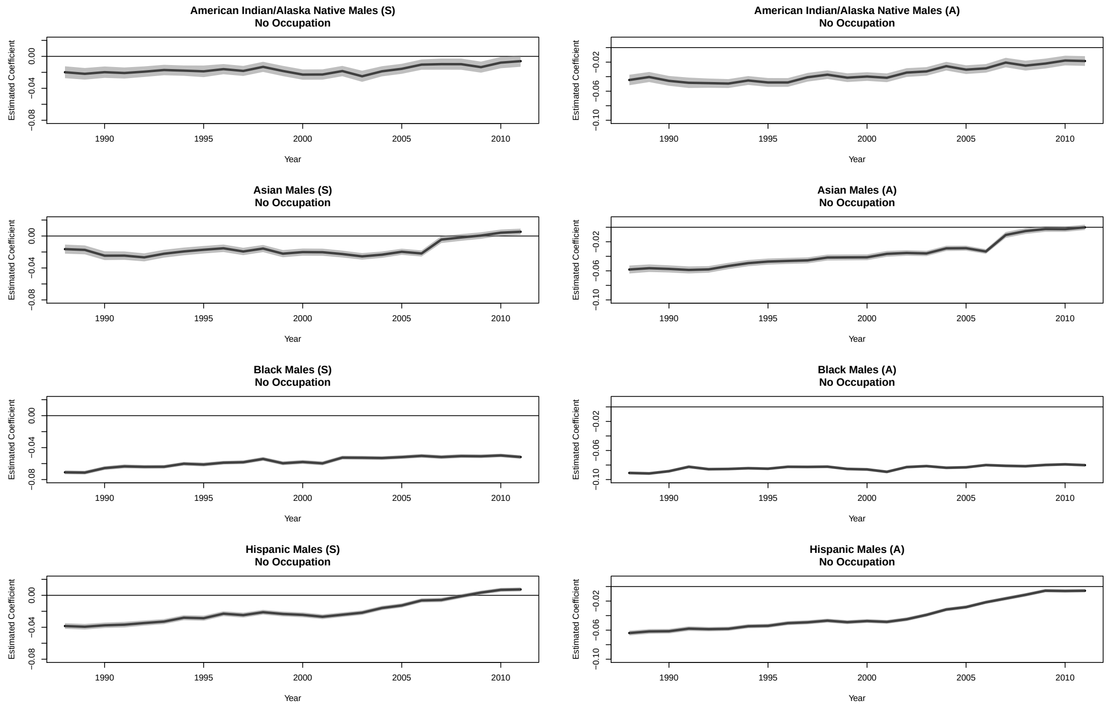


Figure 2: Estimated racial wage gaps (coefficients of race indicators) for yearly males' regressions in synthetic data (left) and confidential, authentic data (right). These models include an indicator for an individual's occupational category code – professional, administrative (omitted category), technical, clerical, other white collar, or blue collar.

is for black female employees, a trend which is replicated in models with more disaggregated occupational information as well. In the confidential dataset, we see a decline in black female earnings relative to whites over time, whereas we see no clear trend in the synthetic dataset estimates. Again, we observe relatively larger magnitude estimates in the confidential datasets.

Figure 2 displays over-time trends and 95% confidence intervals for the racial pay gap for male employees in the federal government. As can be seen, there are relatively similar trends to those reported in the main text of the paper and the results are fairly consistent across the synthetic and the confidential datasets as well. The only sign discrepancy appears to be for Hispanic males, who are estimated to earn more than white males in the latter years of the dataset in the synthetic dataset. This is not replicated in the confidential dataset. There are a couple of minor differences between these results and those reported in the main text. With disaggregated occupational information, we see that Asian male employees appear to reach parity with white male employees in the latter years of the dataset. We also see that in these models, employees who identify as American Indian or Alaska Native also appear to fare less well, never reaching parity, while they do when using disaggregated occupational data.

# 5 Method for empirical disclosure risk assessment for OPM synthetic data

In Section 3.2.5 of the main text, we report results of an empirical disclosure risk assessment. Here, we describe the methodology underpinning that assessment. Specifically, we describe the approach that we used to estimate the probabilities that intruders could learn values of employee's race, one of the most sensitive variables in the OPM SF file, given the synthetic data and other publicly available information. In that section in the main text, we also compare the empirical disclosure risk from the synthetic data to empirical disclosure risk using information from the data cubes. We do not describe the methodology used to estimate the probabilities of learning race from the information in the data cubes. Because the data cubes are public, describing this algorithm in detail would provide a blueprint for intruders to learn many employees' races. While arguably using the public data to learn information is not illegal—after all, the data are public—we do not feel it appropriate to provide this blueprint, as we have promised not to reveal sensitive information as part of the data use agreement with the OPM.

Let $\mathbf{D}_S$ be the fully synthetic version of the Status File described in the main text. We consider employee's race in 2011 as the confidential characteristic of interest; similar methods apply for other sensitive variables. Let $\mathbf{D}_B$ be the publicly available dataset released by BuzzFeed (see, *https://www.buzzfeed.com/*). This comprises federal employees' names and demographic information (other than race and gender) for 2011 and other years. The basic steps of the empirical risk assessment include (i) use $\mathbf{D}_B$ to identify individual employees, (ii) specify a predictive model for race given the characteristics in $\mathbf{D}_B$, (iii) estimate the model using $\mathbf{D}_S$, and (iv) use the predictions as guesses of the actual races for the individuals identified in $\mathbf{D}_B$.

Specifically, we compute the probability of correctly predicting employees' race based on $\mathbf{D}_S$ and $\mathbf{D}_B$ as follows. As conditional variables from $\mathbf{D}_B$, we use agency ($Y_1$), occupation ($Y_2$), occupational category ($Y_3$), age ($Y_4$), educational level ($Y_5$), adjusted basic pay ($Y_6$), pay plan ($Y_7$), pay grade ($Y_8$), type of appointment ($Y_9$), work schedule ($Y_{10}$), and supervisory status ($Y_{11}$). We build a predictive model for race given $(Y_1, \ldots, Y_{11})$ and estimate it with $\mathbf{D}_S$. We then compute $p_{iS}$, the probability of correctly predicting the race of the $i$th employee in $\mathbf{D}_B$ based on $\mathbf{D}_S$, as described in Section 5.1.

We followed a similar process for the disclosure risks when using the information in the data cubes, which we label as $\mathbf{D}_C$. That is, since $\mathbf{D}_C$ contains aggregated information about the reported races ($R$) and $Y_j$, where $j \in \{1, \ldots, 11\}$, we can use $\mathbf{D}_C$ to build a predictive mechanism for race. From this we can compute $p_{iC}$, the probability of correctly predicting the race of the $i$th employee in $\mathbf{D}_B$ based on $\mathbf{D}_C$. We do not describe the predictive model further for reasons described previously. We assess the risk of releasing $\mathbf{D}_S$ to the baseline of releasing $\mathbf{D}_C$ by comparing $p_{iS}$ with $p_{iC}$. In that way, we can evaluate how much information an intruder

can learn about the $i$th employee's race from $p_{iS}$ given that the intruder already can know $p_{iC}$.

### 5.1 Computing $p_{iS}$

By using the synthetic dataset $\mathbf{D}_S$, we can compute, for every race $r$ and every level $y_j$ of $Y_j$, the count

$$N_S(R = r, Y_j = y_j, j \in \{1, \dots, 11\}) = \sum_{l=1}^{n} \mathbb{I}_{\{r\}}(r_l^s) \prod_{j \in \mathcal{I}} \mathbb{I}_{\{y_j\}}(y_{lj}^s),$$

where $r_l^s$ and $y_{lj}^s$ represent the values of reported race $R$ and $Y_j$ associated with the $l$th synthetic employee. Here, $\mathbb{I}_{\{a\}}(b) = 1$ when $a = b$ and equals zero otherwise. The value of $N_S(R = r, Y_j = y_j, j \in \{1, \dots, 11\})$ corresponds to the number of synthetic employees in $\mathbf{D}_S$ that reported race $r$ and $y_j$ for $Y_j$, $j \in \{1, \dots, 11\}$. Thus, we define

$$P_S(R = r | Y_j = y_j, j \in \{1, \dots, 11\}) = \frac{N_S(R = r, Y_j = y_j, j \in \{1, \dots, 11\})}{\sum_{r' \in \mathcal{R}} N_S(R = r', Y_j = y_j, j \in \{1, \dots, 11\})},$$

and

$$p_{iS} = P(R = r_i | Y_j = y_{ij}, j \in \{1, \dots, 11\}),$$

where $r_i$ and $y_{ij}$ represent the values of $R$ and $Y_j$ reported by the $i$th employee in the Status File, and $\mathcal{R}$ = {American Indian or Alaskan Native, Asian, Black/African American, Native Hawaiian or Pacific Islander, Hispanic/Latino, White, Unspecified}. In those cases where, for every $r \in \mathcal{R}$, $N_S(R = r, Y_j = y_j, j \in \{1, \dots, 11\}) = 0$, we define $p_{iS} = 1/7$.

### 5.2 Using the empirical probabilities

We compute and compare the probabilities $p_{iS}$, as well as $p_{iC}$, for $1,353,400$ employees, that is, all employees that worked during 2011. Results of these comparisons show that for less than 6% of the employees, $p_{iC} < 1$ and $p_{iS} = 1$. For these employees, the intruder cannot perfectly predict their race (using our methodology) from $\mathbf{D}_C$ alone; however, the intruder could correctly estimate the race of these employees (using our methodology) if $\mathbf{D}_S$ were released and the intruder used $p_{iS}$ instead of $p_{iC}$. There are far more cases where $p_{iS} < 1$ and $p_{iC} = 1$, suggesting that intruders in general would be better off attacking the data cubes than attacking $\mathbf{D}_S$ to learn employees' races.

## 6 Longitudinal Verification Measure

In addition to verifying whether a given coefficient exceeds some threshold, analysts can also be interested in studying how $\beta_{jt}$ changes across time, where $\beta_{jt}$ is the regression coefficient of interest at year $t$. To study how $\beta_{jt}$ changes across time, we assume that $\mathbf{D}$ can be divided

into nonempty subsets $\mathbf{D}^1, \ldots, \mathbf{D}^{24}$, where $\mathbf{D} = \{(\mathbf{x}_i, y_i)\}_{i=1}^n$, $\mathbf{D}^t$ denotes all the data points in $\mathbf{D}$ observed at year $t$, $y_i \in \mathbb{R}$ is the response variable, and $\mathbf{x}_i = (1, x_{i,1}, \ldots, x_{i,p})^T \in \mathbb{R}^{p+1}$ are the set of predictors. We also assume that, for every $(y_{it}, \mathbf{x}_{it}) \in \mathbf{D}^t$, $E(y_{it}|\mathbf{x}_{it}) = \boldsymbol{\beta}_t^T \mathbf{x}_{it}$, where $\boldsymbol{\beta}_t = (\beta_{0t}, \ldots, \beta_{pt})^T \in \mathbb{R}^{p+1}$. To formally state our goal here, let $m\left(\{(t, \beta_{jt})\}_{t\in\mathcal{T}}\right)$ be a $\{0,1\}$-valued function which returns a zero if the OLS line passing through the points $\{(t, \beta_{jt})\}_{t\in\mathcal{T}}$ has negative slope and returns a one if the slope is positive, where $\mathcal{T}$ is a period of years. Here, we presume the analyst is specifically interested in checking whether $\beta_{jt}$ has an increasing or decreasing trend in a given period of years $\mathcal{T}$, i.e., whether $m\left(\{(t, \beta_{jt})\}_{t\in\mathcal{T}}\right)$ equals zero or one. More generally, we assume the analyst can consider $K$ periods of the form $\mathcal{T}_k = [t_{k-1}, t_k]$, $k = 1, \ldots, K$, where $1 = t_0 < t_1 < \ldots < t_K = 24$, and check whether the trend of $\beta_{jt}$ is increasing or decreasing within each $\mathcal{T}_k$. Hence, for a given sequence $(\tau_1, \ldots, \tau_K) \in \{0,1\}^K$, we can think of the analyst's interest as an inference problem where the parameter to infer is defined by $\theta_0 = \prod_{k=1}^K \mathbb{I}_{\{\tau_k\}}\left(m\left(\{(t, \beta_{jt})\}_{t\in\mathcal{T}_k}\right)\right)$. Notice that $\theta_0$ is a binary parameter such that it is equal to one when $\tau_k = m\left(\{(t, \beta_{jt})\}_{t\in\mathcal{T}}\right)$, for every $k = 1, \ldots, K$, and is equal to zero otherwise. For example, an analysis of whether the trend of $\beta_{jt}$ is decreasing during the first 9 years and is increasing during the last 15 years would examine whether $\theta_0 = 1$ when $(\tau_1, \tau_2) = (0, 1)$, $\mathcal{T}_1 = [1, 9]$, and $\mathcal{T}_2 = [10, 24]$.

Similar to the DP verification procedure for the threshold, and because of the large sample sizes in the SF data, approximated inferences for $\theta_0$ can be made by using a pseudo parameter $\theta_N$. This pseudo parameter is a function of the sampling distribution of the MLE of $\beta_{jt}$, $t = 1, \ldots, 24$. We define the pseudo parameter $\theta_N$ by

$$\theta_{N_1,\ldots,N_{24}} = \begin{cases} 1 & \text{if } P[m(\{(t, \hat{\beta}_{jt}^{N_t})\}_{t\in\mathcal{T}_k}) = \tau_k, k = 1, \ldots, K] \geq \gamma_1, \\ 0 & \text{if } P[m(\{(t, \hat{\beta}_{jt}^{N_t})\}_{t\in\mathcal{T}_k}) = \tau_k, k = 1, \ldots, K] < \gamma_1. \end{cases}$$

where $\hat{\beta}_{jt}^{N_t}$ is the MLE of $\beta_{jt}$ based on a sample with $N_t$ individuals and, again, $\gamma_1 \in (0,1)$ reflects the degree of certainty the user requires before she decides there is enough evidence to conclude that $\theta_0 = 1$. In this case, if $\hat{\beta}_{jt}^{N_t}$ is a consistent estimator of $\beta_{jt}$, we have that $\lim_{\forall t, N_t\to\infty} \theta_{N_1,\ldots,N_{24}} = \theta_0$.

Since making inferences about $\theta_{N_1,\ldots,N_{24}}$ is equivalent to making inferences about $r = P[m(\{(t, \hat{\beta}_{jt}^{N_t})\}_{t\in\mathcal{T}_k}) = \tau_k, k = 1, \ldots, K]$, we focus on providing a DP procedure for releasing inferences for $r$. This procedure is based on the subsample and aggregate method. We start by randomly splitting each $\mathbf{D}^t$ into $M$ disjoint subsets, $\mathbf{D}_1^t, \ldots, \mathbf{D}_M^t$, of the same size (or approximately the same size when $n_t/M$ is not an integer with $n_t = |\mathbf{D}^t|$), where $M$ is specified by the user. Then, in each $D_l^t$, we compute the MLE $b_{jtl}$ of $\beta_{jt}$. We assume that, for each $t$, $b_{jt1}, \ldots, b_{jtM}$ is a random sample from the sampling distribution of $\hat{\beta}_{jt}^{N_t}$, where $N_t = n_t/M$. Let $W_l = \prod_{k=1}^K \mathbb{I}_{\{\tau_k\}}(m\left(\{(t, b_{jtl})\}_{t\in\mathcal{T}_k}\right)$ and $S = \sum_{l=1}^M W_l$. Since $W_1, \ldots, W_M$ are independent Bernoulli distributed random variables with parameter $r$, we can provide inferences for $r$ by using the Binomial random variable $S$.

Unfortunately, inferences directly based on $S$ can lead to leakage of information. Hence, we propose to make inferences for $r$ based on a DP version of $S$, say $S^R = S + \eta$, where $\eta$ is drawn from a Laplace distribution with mean zero and variance $1/\epsilon$.

Based on $S^R$, we make inferences for $r$ by using the following model,

$$S^R|S \sim \text{Laplace}(S, 1/\epsilon), \quad S \mid r \sim \text{Binomial}(M, r), \quad r \sim \text{Beta}(1, 1).$$

Under this model, the verification server can report back any graph or summary of the posterior distribution of $r$ to the analyst. Then, she can compare any of those outputs with her degree of certainty represented by $\gamma_1$ and decides whether or not $\theta_0 = 1$. She can alternatively interpret this posterior distribution for $r$ as an asymptotic approximation of the Bayesian posterior probability, $\pi(m(\{(t, \beta_{jt})\}_{t \in \mathcal{T}_k}) = \tau_k, k = 1, \ldots, K|S^R)$. In our previous example where $(\tau_1, \tau_2) = (0, 1)$, $\mathcal{T}_1 = [1, 9]$, and $\mathcal{T}_2 = [10, 24]$, if the mode of the posterior probability for $r$ equals 0.93, we could say that the posterior probability that the trend of $\beta_{jt}$ is decreasing during the first 9 years and is increasing during the last 15 years is approximately equal to 0.93.

# 7 Further details on the differentially private verification measures

In this section, we further examine the performance of the $\epsilon$-differentially private verification measure for regression coefficients described in Section 4.1 of the main text. Specifically, we empirically investigate how the measures perform under different values of $M$ and $\epsilon$, two key inputs to the verification algorithm. We also examine the performance under different features of the data, the other key input to the algorithm. In section 7.1, we review and define quantities involved in the verification measure. We provide intuition on how these quantities can influence the performance of the verification measure. In section 7.2, we describe a modification of the verification measure that is suitable for analyses where some regression coefficients are nonestimable. In section 7.3, we examine the performance of the original and modified verification measures using the confidential OPM data, focusing on analyses of race gaps in pay in particular agencies and occupations.

## 7.1 Quantities influencing verification measures

In the $\epsilon$-differentially private verification measure described in Section 4.1 of the main text, analysts seek to assess whether or not the value of a regression coefficient $\beta_j$ exceeds some threshold $\gamma_0$. The measure uses the subsample and aggregate method proposed by Nissim et al. (2007). This method requires spliting the confidential data $\mathbf{D}$ into $M$ disjoint subsets, where $M$ is selected by the data analyst. We note that the data analyst generally does not select $\epsilon$, as $\epsilon$

is determined by the policies of the data steward.

The values of $M$ and $\epsilon$ affect the measure's performance. All else being equal, reducing $\epsilon$ (which strengthens the privacy guarantees) increases the variance in the Laplace distribution used in the verification measure. In turn, this degrades the usefulness of the measure. The effects of changing $M$, however, are more subtle. On the one hand, $M$ controls the sensitivity of the verification measure: the larger the $M$, the lower the sensitivity and vice-versa. Lowering sensitivity translates to decreasing the variance of the Laplace distribution, and therefore increasing the usefulness of the measure. On the other hand, the effects of changing $M$ depend on the sample size $n$ of the data $\mathbf{D}$ used in the verification request, as well as the number of observations $n_j$ in $\mathbf{D}$ available to estimate $\beta_j$. As an example of $n_j$, when $\beta_j$ is associated with American Indian/Alaska Native race in the wage gap regressions of Section 5 in the main text, $n_j$ is the number of employees who chose to identify with that race. By splitting $\mathbf{D}$ into $M$ subsets $\mathbf{D}_1, \ldots, \mathbf{D}_M$, we increase the standard errors of the estimates of $\beta_j$ within the subsets. When $N = M/n$ is small, the increase in these standard errors can complicate interpretation of the measures. For example, if these standard errors are very large, the estimates of $\beta_j$ in the partitions could be very dispersed, making it difficult to interpret what the measure (even without the Laplace noise) says about $\beta_j$. We demonstrate these issues empirically in Section 7.3.

## 7.2 Verification with potentially nonestimable regression coefficients

In some cases, analysts can end up not having observations to estimate $\beta_j$ within some subsets. That is, for some $\mathbf{D}_l$ we have $n_{lj} = 0$, where $n_{lj}$ is the number of observations in $\mathbf{D}_l$ available to estimate $\beta_j$. Alternatively, $\beta_j$ can be nonestimable in partitions $\mathbf{D}_l$ that do not have sufficient information to estimate the intercept of the regression model. This could happen if $\mathbf{D}_l$ does not contain observations for at least one of the reference levels of categorical predictors. When $\beta_j$ is nonestimable from $\mathbf{D}_l$, most regression software (including $R$) produce an error when attempting to compute $b_{jl}$, where $b_{jl}$ is the MLE estimate of $\beta_j$ computed from $\mathbf{D}_l$.

Motivated by the nonestimability of $\beta_j$ for some $\mathbf{D}_l$, we provide a modified verification measure for $\beta_j$ intended to deal with this problem. Specifically, we report, in a differentially private way, two quantities: the number of $b_{jl}$ that we are not able to estimate, and the fraction of estimable $b_{jl}$ that exceed $\gamma_0$. We now describe the modified verification measure for $\beta_j$.

Similarly to Section 4.1 of the main text, we aim to infer whether or not $\theta_0 = \mathbb{I}_{(-\infty,\gamma_0]}(\beta_j)$ is equal to zero or one, where $\beta_j$ is a coefficient associated with a level of a categorical variable. To do so, we plan to approximate $\theta_0 = \mathbb{I}_{(-\infty,\gamma_0]}(\beta_j)$ by using the pseudo-parameter,

$$\theta_N = \begin{cases} 1 & \text{if } P(\hat{\beta}_j^N \leq \gamma_0 | \hat{\beta}_j^N \neq \texttt{NA}\ ) \geq \gamma_1, \\ 0 & \text{if } P(\hat{\beta}_j^N \leq \gamma_0 | \hat{\beta}_j^N \neq \texttt{NA}) < \gamma_1, \end{cases}$$

where $\hat{\beta}_j^N$ is the MLE of $\beta_j$ based on a sample with $N$ individuals (where $N$ stands for a generic sample size). Here, $\gamma_1 \in (0,1)$ reflects the degree of certainty required by the user before she decides there is enough evidence to conclude that $\theta_0 = 1$. We also assume that $\hat{\beta}_j^N \in \mathbb{R} \cup \{\texttt{NA}\}$, where NA represents the nonestimability condition. Recall that $\hat{\beta}_j^N = \texttt{NA}$ if, for example, $n_j = 0$. When $\hat{\beta}_j^N$ is a consistent estimator of $\beta_j$, we can guarantee that $\lim_{N\to\infty} \theta_N = \theta_0$ if $\lim_{N\to\infty} P(\hat{\beta}_j^N \neq \texttt{NA}) = 1$.

Unfortunately, we cannot release $\hat{\beta}_j^N$, nor other deterministic functions of $\mathbf{D}$, directly. Instead, we release a noisy version of the key quantity in $\theta_N$, namely $\mathbf{q} = (q_1, q_0, q_{\texttt{NA}}) = (P(\hat{\beta}_j^N \leq \gamma_0), P(\hat{\beta}_j^N > \gamma_0), P(\hat{\beta}_j^N = \texttt{NA}))$. We do so using the sub-sample and aggregate method (Nissim et al., 2007). We randomly split $\mathbf{D}$ into $M$ disjoint subsets, $\mathbf{D}_1, \ldots, \mathbf{D}_M$, of size $N$ (with inconsequential differences when $N = n/M$ is not an integer), where $M$ is selected by the user. In each $\mathbf{D_l}$, where $l = 1, \ldots, M$, we attempt to compute the MLE $b_{jl}$ of $\beta_j$. The $(b_{j1}, \ldots, b_{jM})$ can be treated as $M$ independent draws from the distribution of $\hat{\beta}_j^N$, where $N = n/M$. Let $\mathbf{W}_l = (\mathbb{I}_{(-\infty,\gamma_0]}(b_{jl}),\ \mathbb{I}_{(\gamma_0,\infty)}(b_{jl}),\ \mathbb{I}_{\texttt{NA}}(b_{jl}))$. Each $W_l$ is an independent, multinomial distributed random variable with parameters one and $\mathbf{q}$. Thus, inferences for $\mathbf{q}$ can be made based on $\mathbf{S} = (S_1, S_2, S_3) = \sum_{l=1}^M \mathbf{W}_l$; that is, we sum up the number of partitions with estimable $b_{jl}$ that exceed the threshold, with estimable $b_{jl}$ that do not exceed the threshold, and where $\beta_j$ cannot be estimated. We cannot release $\mathbf{S}$ directly and satisfy $\epsilon$-DP; instead, we generate a noisy version of $\mathbf{S}$ using the Laplace Mechanism with $\lambda = 2/\epsilon$, resulting in $\mathbf{S}^R = \mathbf{S} + \boldsymbol{\eta}$. The global sensitivity equals 2, since at most two components of $\mathbf{S}$ can change by at most one unit.

The noisy $\mathbf{S}^R$ satisfies $\epsilon$-DP; however, interpreting it directly can be tricky. First, the components of $\mathbf{S}^R$ are not guaranteed to lie in $(0, M)$ nor even to be an integer and to add to $M$. Second, alone $\mathbf{S}^R$ does not provide estimates of uncertainty about $\mathbf{q}$. We therefore use a post-processing step—which has no bearing on the privacy properties of component of $\mathbf{S}^R$—to improve interpretation. We find the posterior distribution of $\mathbf{q}$ conditional on $\mathbf{S}^R$ and using the noise distribution, which is publicly known. Using simple MCMC techniques, we estimate the model,

$$\mathbf{S}^R | \mathbf{S} \sim \text{Laplace}_3(\mathbf{S}, 2/\epsilon), \quad \mathbf{S} \mid \mathbf{q} \sim \text{Binomial}(M, \mathbf{1}), \quad \mathbf{q} \sim \text{Dirichlet}(1,1,1), \tag{5}$$

where $\text{Laplace}_3$ denote the multivariate distribution induced by three independent univariate Laplace distributions with location and scale parameters determined by $\mathbf{S}$ and $2/\epsilon$. Here, we treat $\mathbf{S}$ as an unobserved random vector and average over it.

The verification server reports back the posterior distribution of $\mathbf{q}$ to the analyst, who can approximate $\theta_N$ for any specified $\gamma_1$ simply by finding the amount of posterior mass below $\gamma_1$. Alternatively, analysts can interpret, for example, the posterior distribution for $q_1/(q_1 + q_0)$ as a crude approximation to the Bayesian posterior probability, $\pi\left(\beta_j \leq \gamma_0 | \mathbf{S}^R\right)$. For instance, if the posterior mode for $q_1/(q_1 + q_0)$ equals 0.87, we could say that the posterior probability

that $\beta_j < \gamma_0$ is approximately equal to 0.87. Finally, the analyst can use $q_{\texttt{NA}}$ to quantify the estimability of $\hat{\beta}_j$ among the subsets $\mathbf{D}_1, \ldots, \mathbf{D}_M$. We caution that the analyst should refrain from providing conclusions based on $q_1/(q_1+q_0)$ on those cases where $q_{\texttt{NA}}$ is large, say more than 20%.

### 7.3 Empirical study

In this section, we present an empirical study of the the verification measures proposed in section 7.2 and section 4.1 of the main text. Hereafter, we refer to these measures as multinomial-based and binomial-based measures, respectively. We perform the empirical analysis to illustrate how different values of $(\epsilon, M, n, n_j)$ affect the performance of the verification measures, to compare the usefulness of the two proposed verification measures, and to identify and design strategies that guide analysts to use and interpret the verification measures more effectively. Given access to the synthetic data, analysts can use the synthetic data to do similar experiments for their particular analyses of interest to assess whether or not the verification measures are likely to return useful information for those analyses.

In the empirical study, we consider seven subsets of the Status File by splitting on agency, occupation, and sex. The seven subsets are displayed in Table 2. We select these subsets to cover a range of values of $n$ and $n_j$. For each subset, we perform an overall regression analysis similar to the one described in section 5.3 of the main text. Each observation is an employee-year. The dependent variable is the natural logarithm of each employee's inflation adjusted basic pay in a given year. The key independent variable is the race with which individual employees identify. While we include other independent variables such as employees' age as well as its square, and years of education, we input only race coefficients into the verification algorithms.

For each subset, we perform the regression analysis on the confidential data and record the estimated coefficients. We run the multinomial-based and binomial-based measures using three values of $\epsilon \in \{.5, 1, 2\}$ and three values of $M \in \{10, 30, 50\}$. We use the algorithms to verify whether or not estimated coefficients are below the threshold of $-0.01$. For each subset and combination of $(\epsilon, M)$, we run the verification algorithms ten times, each time generating new partitions and Laplace noise. We report average values and standard errors of $\hat{r}$ for the binomial-based measure and $\hat{q}$ for the multinomial-based measure, where $\hat{r}$ and $\hat{q}$ are the posterior modes of $r$ and $q_1/(q_1+q_0)$, respectively. More precisely, we query ten times $\hat{r}$ and $\hat{q}$ and report average values of the form

$$\frac{1}{10}\sum_{i=1} \hat{r}^{(i)} \text{ and } \frac{1}{10}\sum_{i=1} \hat{q}^{(i)}, \tag{6}$$

| Scenario | Agency | Occupation | Sex | Race | $n$ | $n_j$ | $\hat{\beta}_j$ |
|---|---|---|---|---|---|---|---|
| 1 | VATA | Practical Nurse | F | Black | 193,144 | 66,394 | 0.02 |
| 2 | SZ00 | Social Insurance Admin. | F | Hispanic | 305,311 | 42,709 | -0.04 |
| 3 | TD03 | Air Traffic Control | M | Black | 458,114 | 21,416 | -0.05 |
| 4 | TR93 | Tax Examining | F | Asian | 165,210 | 3,963 | -0.03 |
| 5 | DJ09 | General Attorney | F | Black | 34,154 | 3,748 | -0.01 |
| 6 | DJ02 | Criminal Investigating | F | Asian | 42,077 | 1,225 | -0.04 |
| 7 | LF00 | General Attorney | F | Asian | 705 | 32 | -0.05 |

Table 2: Scenario definitions for empirical study of verification measures. Agency, occupation, and sex define the subset of the Status File to be analyzed. Race determines the coefficient to be verified and $\hat{\beta}_j$ its corresponding MLE estimate. The considered agencies are Veterans Health Administration (VATA), Social Security Administration (SZ00), Federal Aviation Administration (TD03), Internal Revenue Service (TR93), Office of U.S. Attorney (DJ09), Federal Bureau of Investigation (DJ02), and Federal Election Commission (LF00). $n$ denotes the number of employees in each subset and $n_j$ indicates the number of employees identifying with the displayed race (fifth column). $\hat{\beta}_j$ provides the coefficient estimates from regression models with the confidential data.

and standard errors of the form

$$\left(\frac{1}{9}\sum_{i=1}\left(\hat{r}^{(i)}-\frac{1}{10}\sum_{l=1}\hat{r}^{(l)}\right)^2\right)^{1/2} \text{ and } \left(\frac{1}{9}\sum_{i=1}\left(\hat{q}^{(i)}-\frac{1}{10}\sum_{l=1}\hat{q}^{(l)}\right)^2\right)^{1/2}, \tag{7}$$

where $\hat{r}^{(i)}$ and $\hat{q}^{(i)}$ denotes the value of $\hat{r}$ and $\hat{q}$ obtained in the $i$-th query.

Table 3 displays the average values over ten queries of $\hat{r}$ and $\hat{q}$ for all scenarios and values of $\epsilon$ and $M$. We start by analyzing the results for scenario 7, which has a very small value of $n_j$. Here, the coefficient for race is below the threshold, so a useful verification measure should report large values of $\hat{r}$. However, because the number of employees who identify as Asian is quite small, the subsample and aggregate method often leads to subsets having no or few employees who identify as Asian. With the high frequency of errors, typically we cannot compute $\hat{r}$ for the binomial-based measure. For the multinomial-based measure, $\hat{q}$ is typically around .5, reflecting the fact that we cannot tell if it is above or below the threshold. Apparently, for scenarios with very small $n_j$, the verification measure generally cannot be relied on to help analysts decide that coefficients are below thresholds.

We next turn to scenario 5. Here, $n_j$ is large enough to make it unlikely that we get partitions where the coefficient of interest is inestimable. The estimate in the confidential data is approximately equal to the threshold, so we would expect $\hat{r}$ and $\hat{q}$ to be around .5. This result is confirmed in Table 3. For this scenario, there are no obvious patterns in the average values of $\hat{r}$ and $\hat{q}$ across the different combinations of $M$ and $\epsilon$.

Scenarios 1, 2, 3, 4, and 6 have reasonably large values for $n_j$ and coefficients unambiguously

above or below the thresholds. For these scenarios, the average values of $\hat{r}$ and $\hat{q}$ tend to provide useful verifications of the tested conditions across all values of $M$ and $\epsilon$ examined here, being small when the true coefficient is above the threshold and large when it is below the threshold. The results from these scenarios also shed light on how $(\epsilon, M, n, n_j)$ impact the performance of the verification measures. Broadly, it is apparent that the effects are interactive; for example, making $M = 50$ can be optimal for one sample size but not another, or at one level of $\epsilon$ but not another.

Considering $\epsilon$ first, we see the effects on accuracy of decreasing $\epsilon$ most noticeably when $M = 10$. With the larger sample sizes these effects are modest; for example, when going from $\epsilon = 2$ to $\epsilon = .5$, in Scenario 2 we drop from a .98 average $\hat{r}$ to a .94 average $\hat{r}$. With the smaller sample sizes these effects are more substantial; for example, when going from $\epsilon = 2$ to $\epsilon = .5$, in Scenario 3 we drop from a .98 average $\hat{r}$ to a .81 average $\hat{r}$. When $M \geq 30$, the effects of going from $\epsilon = 2$ to $\epsilon = .5$ are not practically important. This is encouraging news, as verifications that use smaller $\epsilon$ consume less of the privacy budget.

Turning to $M$, we find differential effects across scenarios 1, 2, 3, 4, and 6. For the large $n$ scenarios 1 and 2, when $\epsilon = .5, 1$, the averages of $\hat{r}$ are similar when one uses $M = 30$ or $M = 50$. Using $M = 10$ in these cases degrades the average $\hat{r}$ somewhat, as the averages shrink toward 0.5 which is away from the ideal verification values in these scenarios. We find similar patterns for $\hat{q}$. For scenario 3, we see that the optimal value of $M$ depends on the value of $\epsilon$. We prefer $M = 10$ when $\epsilon = 1,\ 2$, and we prefer $M = 30$ when $\epsilon = .5$. We see similar patterns for scenario 4. For scenario 6, which has a relatively small $n_j$, we see that $M = 10$ provides the optimal usefulness of the verification measure. For cases where $M = 10$ is optimal, using larger values of $M$ increases the standard error of the estimated coefficients within the partitions, causing them to fall above the threshold with high enough chance so as to degrade the performance of the verification measures.

In many cases in Table 3, measures behave differently as a function of $M$ when $\epsilon = .5$ and $\epsilon = 1,\ 2$. This is not surprising, actually. Setting $\epsilon = .5$ encourages the Laplace distribution to inject more noise. This is counterbalanced by increasing $M$, since the variance in the Laplace noise is proportional to $1/M\epsilon$. However, increasing $M$ also increases standard errors, which can result in higher fractions of the estimated coefficients in the partitions not satisfying the threshold condition.

Accuracy also depends on whether we use the binomial-based or multinomial-based strategy. The absolute difference between average values of $\hat{r}$ and $\hat{q}$ decreases as $\epsilon$ increases; maximum differences are .07, .05, and .03 when $\epsilon$ is .5, 1, and 2, respectively. These observed differences should have low impacts on how analysts interpret verification measures, suggesting that, for scenarios like 1, 2, 3, 4, and 6, $\hat{r}$ and $\hat{q}$ have roughly the same usefulness. Of course, we cannot meaningfully use $\hat{r}$ when there are errors in some partitions, whereas we can use $\hat{q}$. One way to

| | | | | $\epsilon = .5$ | | $\epsilon = 1$ | | $\epsilon = 2$ | |
|---|---|---|---|---|---|---|---|---|---|
| E | $\hat{\beta}_j$ | $S_1$ | $M$ | $\hat{r}$ | $\hat{q}$ | $\hat{r}$ | $\hat{q}$ | $\hat{r}$ | $\hat{q}$ |
| | | 0 | 10 | .07 (.066) | .09 (.070) | .04 (.061) | .11 (.193) | .04 (.063) | .02 (.022) |
| 1 | .02 | 0 | 30 | .03 (.051) | .04 (.052) | .01 (.016) | .04 (.044) | .01 (.014) | .01 (.003) |
| | | .3 | 50 | .03 (.035) | .02 (.016) | .02 (.027) | .01 (.014) | .01 (.017) | .01 (.008) |
| | | 10 | 10 | .94 (.088) | .84 (.155) | .93 (.073) | .92 (.071) | .98 (.023) | .96 (.042) |
| 2 | -.04 | 29.5 | 30 | .95 (.055) | .97 (.021) | .98 (.018) | .98 (.011) | .98 (.026) | .98 (.016) |
| | | 47.5 | 50 | .97 (.032) | .98 (.010) | .96 (.022) | .97 (.028) | .95 (.020) | .97 (.025) |
| | | 10 | 10 | .81 (.243) | .76 (.250) | .94 (.092) | .98 (.009) | .98 (.031) | .96 (.043) |
| 3 | -.05 | 27.7 | 30 | .89 (.095) | .90 (.119) | .93 (.051) | .92 (.057) | .91 (.047) | .93 (.037) |
| | | 41.1 | 50 | .78 (.081) | .84 (.101) | .81 (.056) | .79 (.085) | .82 (.038) | .82 (.039) |
| | | 9 | 10 | .73 (.310) | .69 (.341) | .85 (.093) | .84 (.232) | .91 (.058) | .93 (.085) |
| 4 | -.03 | 23.1 | 30 | .80 (.107) | .75 (.103) | .77 (.071) | .82 (.114) | .77 (.060) | .77 (.077) |
| | | 36.8 | 50 | .74 (.048) | .78 (.071) | .74 (.041) | .75 (.051) | .74 (.029) | .76 (.049) |
| | | 4.7 | 10 | .55 (.282) | .50 (.292) | .46 (.159) | .58 (.216) | .46 (.073) | .43 (.118) |
| 5 | -.01 | 14.3 | 30 | .49 (.128) | .47 (.156) | .49 (.046) | .46 (.088) | .48 (.043) | .48 (.046) |
| | | 24.7 | 50 | .46 (.066) | .47 (.072) | .48 (.043) | .48 (.056) | .50 (.037) | .49 (.048) |
| | | 8.6 | 10 | .83 (.232) | .81 (.172) | .88 (.077) | .92 (.078) | .88 (.076) | .84 (.092) |
| 6 | -.04 | 22.3 | 30 | .76 (.062) | .73 (.163) | .72 (.086) | .77 (.085) | .75 (.033) | .74 (.033) |
| | | 35.8 | 50 | .69 (.037) | .76 (.081) | .72 (.060) | .72 (.051) | .72 (.032) | .74 (.041) |
| | | 2.8 | 10 | NA | .45 (.309) | NA | .70 (.259) | NA | .62 (.289) |
| 7 | -.05 | 3.7 | 30 | NA | .42 (.310) | NA | .48 (.314) | NA | .56 (.249) |
| | | 3.2 | 50 | NA | .62 (.238) | NA | .62 (.265) | NA | .63 (.273) |

Table 3: Average posterior modes $\hat{r}$ and $\hat{q}$ for all scenarios, $\epsilon \in \{.5, 1, 2\}$ and $M \in \{10, 30, 50\}$. $\hat{\beta}_j$ provides the coefficient estimates from overall regression models. $S_1$ reports the average number of coefficient estimates below the threshold. Standard errors for the posterior modes $\hat{r}$ and $\hat{q}$ are in parentheses. Averages and standard errors are computed over ten queries. We cannot compute $\hat{r}$ in scenario 7 because of the high rate of partitions with errors.

make $\hat{r}$ usable in settings with errors is to randomly set values of partition indicators to zero or one (with equal probability) for partitions with errors.

Table 3 also displays standard errors over the ten queries for $\hat{r}$ and $\hat{q}$ in each scenario. As expected, typically standard errors decrease or stay similar as $\epsilon$ increases. We observe a similar pattern when $M$ increases. Apparently, in these simulations, as $M$ increases the rate at which the variance of the Laplace mechanism decreases is faster than the rate at which the variance of the estimator of $\beta_j$ increases within partitions. For $\epsilon = 0.5$, several standard errors are fairly large, especially when $M = 10$. For $\epsilon = 1, 2$, standard errors tend to be small except when $M = 10$, which can have standard errors up to .232. Finally, we notice that standard errors for the multinomial-based measure typically are larger than those for the binomial-based measure. This is expected, since the multinomial-based measure releases more information, meaning that more error needs to be added to the outcome to protect privacy.

| Scenario | $n$ | $n/n_j$ | $S_1$ | $S_0$ | $S_{\texttt{NA}}$ | $M$ | $q_{\texttt{NA}}$ $\epsilon = .5$ | $\epsilon = 1$ | $\epsilon = 2$ |
|---|---|---|---|---|---|---|---|---|---|
| | | | 0 | 10 | 0 | 10 | .06 (.074) | .08 (.092) | .04 (.045) |
| 1 | 193144 | .34 | 0 | 30 | 0 | 30 | .04 (.064) | .03 (.034) | .01 (.011) |
| | | | .3 | 49.7 | 0 | 50 | .01 (.018) | .02 (.028) | .01 (.005) |
| | | | 10 | 0 | 0 | 10 | .05 (.050) | .03 (.039) | .03 (.038) |
| 2 | 305311 | .14 | 29.5 | .5 | 0 | 30 | .03 (.022) | .01 (.016) | .02 (.014) |
| | | | 47.5 | 2.5 | 0 | 50 | .04 (.040) | .01 (.006) | .01 (.012) |
| | | | 10 | 0 | 0 | 10 | .03 (.015) | .04 (.051) | .05 (.048) |
| 3 | 458114 | .05 | 27.7 | 2.3 | 0 | 30 | .01 (.009) | .02 (.015) | .01 (.012) |
| | | | 41.1 | 8.9 | 0 | 50 | .02 (.020) | .01 (.012) | .01 (.011) |
| | | | 9 | 1 | 0 | 10 | .18 (.218) | .04 (.024) | .05 (.082) |
| 4 | 165210 | .02 | 23.1 | 6.9 | 0 | 30 | .04 (.053) | .05 (.047) | .01 (.004) |
| | | | 36.8 | 13.2 | 0 | 50 | .02 (.033) | .01 (.004) | .01 (.016) |
| | | | 4.7 | 5.3 | 0 | 10 | .06 (.049) | .06 (.082) | .01 (.005) |
| 5 | 34154 | .11 | 14.3 | 15.7 | 0 | 30 | .03 (.060) | .02 (.016) | .01 (.021) |
| | | | 24.7 | 25.3 | 0 | 50 | .07 (.071) | .01 (.010) | .01 (.013) |
| | | | 8.6 | 1.4 | 0 | 10 | .12 (.134) | .06 (.091) | .04 (.036) |
| 6 | 42077 | .03 | 22.3 | 7.7 | 0 | 30 | .09 (.085) | .04 (.053) | .02 (.021) |
| | | | 35.8 | 13.7 | .5 | 50 | .07 (.102) | .03 (.029) | .01 (.014) |
| | | | 2.8 | 2.3 | 4.9 | 10 | .24 (.232) | .44 (.171) | .41 (.132) |
| 7 | 705 | .05 | 3.7 | 3.1 | 23.2 | 30 | .75 (.089) | .75 (.047) | .75 (.066) |
| | | | 3.2 | 2.2 | 44.6 | 50 | .85 (.061) | .87 (.041) | .87 (.031) |

Table 4: Average posterior modes $\hat{q}_{\texttt{NA}}$ for all scenarios, $\epsilon \in \{.5, 1, 2\}$ and $M \in \{10, 30, 50\}$. $S_1$ and $S_0$ report the average number of coefficient estimates below and above the threshold, respectively. $S_{\texttt{NA}}$ displays the average number of nonestimable coefficients. Standard errors for the posterior modes $\hat{q}_{\texttt{NA}}$ are in parentheses. Averages and standard errors are computed over ten queries.

The multinomial-based strategy provides a mean to retrieve, using differential privacy, the proportion of nonestimable regression coefficients within a partition of size $M$. Recall from section 7.2 that we denote this proportion by $q_{\texttt{NA}}$. Table 4 displays the average values and standard errors over ten runs of the posterior modes of $q_{\texttt{NA}}$, denoted by $\hat{q}_{\texttt{NA}}$, for all scenarios and values of $(\epsilon, M)$. We compute theses average values and standard errors using expressions similar to (6) and (7). For the first six scenarios, we observe that errors are extremely rare with these partition sizes. As either $M$ or $\epsilon$ increases, the average $\hat{q}_{\texttt{NA}}$ decreases with few exceptions when epsilon is .5. The magnitude of $\hat{q}_{\texttt{NA}}$ for these scenarios is always small. For Scenario 7, as expected, as $M$ increases so does $\hat{q}_{\texttt{NA}}$. In fact, for $M = 50$, we observe $\hat{q}_{\texttt{NA}}$ around .86, which are fairly large values. Thus, $\hat{q}_{\texttt{NA}}$ fulfills its role of adequately informing about the estimability of the coefficient. Regarding standard errors, we observe some large values particularly when $\epsilon = .5$ or $M = 10$. However, most of the times, the size of standard errors decreases as the value of $\epsilon$ and $M$ increases.

Results reported in Table 3 and Table 4 show how the performance of the verification measures can vary as a function of $\epsilon$, $M$, $n$, and $n_j$. In general, when the values of $n$ and $n_j$ are not small, for the values of $\epsilon$ and $M$ considered here, the binomial-based and multinomial-based measures provide accurate verifications. As a general guideline for $M$, we recommend setting $M > 10$. When analysts have a synthetic dataset, they can find reasonable values for $\epsilon$ and $M$ by computing, for different values of $M$ (and $\epsilon$ when given a choice), the verification measures many times to assess likely performance. When an analyst can find a value of $M$ that works well with the synthetic dataset for the query of interest and allowed $\epsilon$, she can use that value to submit a query for verification based on the confidential file. While this $M$ won't necessarily be optimal, it is likely to be reasonable (when the relationships in the synthetic data reasonably approximate those in the confidential data).

Finally, the multinomial based strategy gives analysts an extra tool to judge whether or not to rely on a requested verification. Specifically, analysts should refrain from using $\hat{q}$ when $\hat{q}_{\texttt{NA}}$ is large. We suggest not relying on the verification measures when the number of errors is 50% or more, as this indicates that the estimates in the partitions are truly too variable to be useful.

## References


K. Nissim, S. Raskhodnikova, and A. Smith. Smooth sensitivity and sampling in private data analysis. In *Proceedings of the thirty-ninth annual ACM symposium on Theory of computing*, pages 75–84. ACM, 2007.

Office of Personnel Management. The guide to data standards, part a: Human resources. Technical report, Office of Personnel Management, 2014.

J. P. Reiter. Using CART to generate partially synthetic, public use microdata. *Journal of Official Statistics*, 21:441–462, 2005.
